# Supplementary material for: Supersampled scanning transmission X-ray microscopy for high-resolution vibration-independent time-resolved imaging
Source: arXiv:2512.17366 ancillary file (2026-05-26)
Supplement: Supplementary file 1 [file SI.pdf]

# Supporting Information: Supersampled scanning transmission X-ray microscopy for high-resolution vibration free imaging

Simone Finizio,<sup>1,\*</sup> Benjamin Watts,<sup>1</sup> Benedikt Rösner,<sup>1</sup> and Jörg Raabe<sup>1</sup>

<sup>1</sup>*Paul Scherrer Institut, 5232 Villigen PSI, Switzerland*

(Dated: December 19, 2025)

## I. SETUP OF THE PANDABOX FPGA

The FPGA of the PandABox data acquisition tool was programmed using the native software of the device, which is structured in separate functional blocks that can be connected together. For the work described here, the following blocks and connections were utilized (refer to the PandABlocks manual [1] for details on the specific block names).

- **CLOCK1:** A 4 kHz clock was configured using the built-in PandABlocks **CLOCK** block. The clock is always enabled.
- **INENC1/2:** Two blocks handling the interferometer input, based on the built-in PandABlocks **INENC** block.
- **PCAP:** Block handling the position capture. The block is always enabled and triggered by the 4 kHz **CLOCK1** block.
- **TTLIN1:** TTL input block, to which the output of the photon counting unit is connected to.
- **TTLIN2:** TTL input block, to which a digital signal set to active when an image is being acquired is connected to.
- **COUNTER1:** A PandABlocks **COUNTER** block, enabled by the **TTLIN2** input, incremented by the **TTLIN1** signal.

The captured position data, together with the **COUNTER1** value, is streamed from the PandABox with a rate defined by **CLOCK1**.

---

\* simone.finizio@psi.ch

## II. DISTRIBUTION OF DWELL TIMES

The binning process described in the main manuscript produces images with a non-constant pixel dwell time, due to the fact that the positioning requirement precision is significantly relaxed if compared to an equivalent constant velocity or point-by-point scan. This implies that the recorded photon counts per pixel need to be normalized by the actual pixel dwell time, and that the quantity that will be displayed in the final image is the photon count rate. The distribution of pixel dwell times in the image depends on several parameters, which affect how the scanning is performed (e.g. scan trajectory, velocity of the stages, etc.). For the scan shown in Fig. 5 of the main manuscript, the distribution of dwell times is displayed in Fig. S1, with a mean pixel dwell time of 38 ms and a standard deviation of 15 ms. Calculations of the Poisson noise will have to take this into consideration.

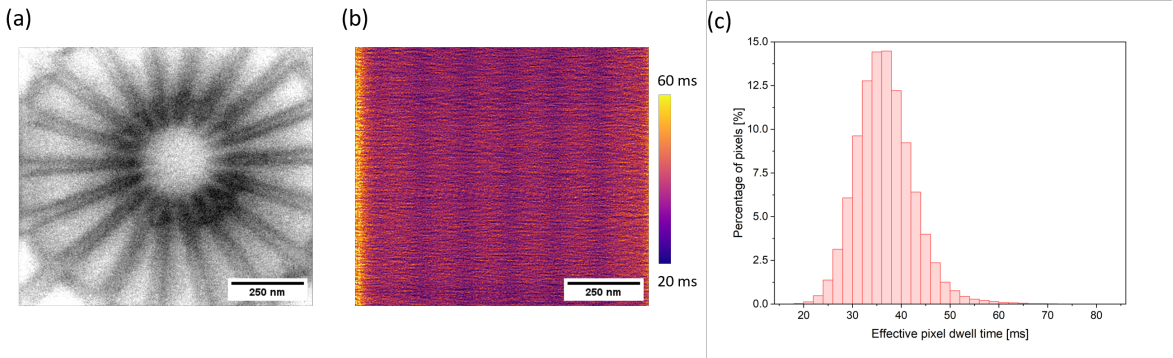

FIG. S1. (a) Supersampled microscopy image of the center region of a 10 nm Ir Siemens star. (b) Map of the total dwell time per pixel. (c) Histogram of the data shown in (b), showing a distribution of dwell times with a mean value of about 38 ms and a standard deviation of about 15 ms.

---

[1] Pandablocks documentation, <https://pandablocks.github.io/PandABlocks-FPGA/master/blocks.html>, accessed: 2025-12-03.
